# Supplementary material for: Hardware Reverse Engineering: Overview and Open Challenges
Source: arXiv:1910.01518 source file (2019-10-01)
Supplement: Supplementary file 1 [file appendix.tex]

% !TEX root = ../main.tex

\appendix

\begin{table*}[!htb]
  \centering
  \begin{tabular}{p{0.05\textwidth}p{0.3\textwidth}p{0.4\textwidth}}
        \Xhline{2\arrayrulewidth}
        & \textbf{Focus} & \textbf{Concepts} \\ \hline
        Process & How do analysts reverse engineer a netlist? & Depending on expertise: Problem solving steps, problem solving strategies, (sub-)goals, use of external sources\\
        Outcome & Did the analyst successfully reverse engineered the correct high-level information? & Accomplishment, knowledge, mental representation, problem solving transfer\\
        Human & What are the prerequisites of the analyst prior to reverse engineering? How strong do theses requirements influence the success of reverse engineering? & Intelligence, resources, expertise, problem solving schemas expertise, prior knowledge \\
        Task & Which characteristics of the task influence the reverse engineering and how strong is their influence? & Amount of gates and signals in the design, complexity of relations between gates, (visual) structure of the gate-level netlist\\
        \Xhline{2\arrayrulewidth}
  \end{tabular}
  \caption{\todo{format and caption}}
  \label{table:appendix}
\end{table*}
